# Supplementary material for: Self-learning analytical interatomic potential describing laser-excited silicon
Source: arXiv:1812.08595 ancillary file (2018-12-20)
Supplement: Supplementary file 1 [file supporting_information.pdf]

# Supporting Information: Self learning analytical interatomic potential describing laser-excited silicon

Bernd Bauerhenne[1,2], Vladimir P. Lipp[1,2,3], Tobias Zier[1,2], Eeuwe S. Zijlstra[1,2], Martin E. Garcia[1,2]

December 20, 2018

[1] Theoretical Physics, University of Kassel, Heinrich-Plett-Straße 40, 34132 Kassel, Germany
[2] Center for Interdisciplinary Nanostructure Science and Technology (CINSaT), Heinrich-Plett-Straße 40, 34132 Kassel, Germany
[3] Current affiliation: Center for Free-Electron Laser Science CFEL, Deutsches Elektronen-Synchrotron DESY, 22607 Hamburg, Germany

Correspondence to: bauerhenne@uni-kassel.de

# Contents

**1 Initial conditions for the *ab initio* MD simulations in thin-film geometry 2**

**2 Iterative procedure to construct a subset of efficient polynomial degrees 2**

**3 Electronic temperature-dependent potential coefficients 3**

**4 Physical properties calculated using the developed interatomic potential 6**

4.1 Atomic root mean-square displacements in $z$-direction . . . . . . . . . . . . 6
4.2 Relative error in forces determined in independent MD simulation runs . . 7
4.3 Absorbed energy of the electrons in the bulk . . . . . . . . . . . . . . . . . . 8
4.4 Electronic absorbed energy and specific heat of an isolated atom . . . . . . 8
4.5 Elastic constants . . . . . . . . . . . . . . . . . . . . . . . . . . . . . . . . . 9
4.6 Pair-correlation function and bond angle distribution . . . . . . . . . . . . 9

**5 Fortran implementation of the developed interatomic potential 11**

# 1 Initial conditions for the *ab initio* MD simulations in thin-film geometry

Initially, we set up a bulk supercell containing 320 Si atoms in the ideal diamond structure with the *ab initio* equilibrium lattice parameter (0.539872 nm) with periodic boundary conditions in all directions. This supercell corresponds to $2 \times 2 \times 10$ primitive cells. We further double the simulation volume by inserting a vacuum in $z$-direction and therefore creating a thin-film. To remove the arising forces at the surface due to unsaturated bonds, we relaxed the atomic coordinates by applying the Fast Inertial Relaxation Engine (FIRE) [2] algorithm in CHIVES. Starting from the obtained relaxed structure of the thin film, we applied the Andersen Thermostat [1] in CHIVES to prepare the ionic temperature of $T_\mathrm{i} = 300$ K. For this, we took true random numbers from `http://www.random.org`.

# 2 Iterative procedure to construct a subset of efficient polynomial degrees

At first, the comprehensive set of errors $\{W\}$ for all physically reasonable degree combinations is calculated using Eq. (6) in the main paper. For this, we consider all possible degree combinations up to the limits of $N_2^{(r)} = 15$, $N_3^{(r)} = 9$, $N_3^{(\theta)} = 9$, $N_\rho^{(\rho)} = 9$, $N_\rho^{(r)} = 9$. For each single degree combination, we find the corresponding optimal cutoff radii which minimize $W$, by testing all cutoff radii in the range between 0.25 nm (which is slightly above the nearest neighbor distance of 0.234 nm) and 0.9 nm with an increment of 0.01 nm. Thus, the comprehensive set contains a large number of combinations of polynomial degrees (potentials), each with the corresponding cutoff radii and the error $W$.
After that, we iteratively construct a subset containing "efficient" polynomial degrees ("efficient" potentials) with relatively low $W$ and relatively low number of coefficients $N_\mathrm{c}$. Note: In the last steps, the used iterative procedure also selects potentials with high $N_\mathrm{c}$. The iterative procedure is initialized at step $k = 0$ with the constant potential $\Phi \equiv \sum_i \Phi_0$, which contains no polynomial coefficients ($N_\mathrm{c} = 0$) and exhibits, by definition, the error of $W = 1$:

$$W^{(0)} = 1, \qquad N_\mathrm{c}^{(0)} = 0. \tag{1}$$

The interatomic potential for each next step $k = 1, 2, \ldots$ is selected among all potentials with $N_\mathrm{c}^{(k)} > N_\mathrm{c}^{(k-1)}$ such that it maximizes the error reduction per number of added coefficients,

$$\frac{W^{(k-1)} - W^{(k)}}{N_\mathrm{c}^{(k)} - N_\mathrm{c}^{(k-1)}} = \frac{\Delta W}{\Delta N_\mathrm{c}}. \tag{2}$$

If the maximal $\Delta W/\Delta N_\mathrm{c}$ is exhibited by several potentials, the one with the smallest number of coefficients $N_\mathrm{c}$ among them is selected. If even $N_\mathrm{c}$ are equal among them, then the potential is randomly selected from them. The procedure stops formally, after the potential with the highest available number of coefficients is selected. At each step $k > 0$, apart from the currently chosen potential, we additionally add to the subset all potentials,

which exhibit an up to 10% smaller $\Delta W/\Delta N_{\mathrm{c}}$. (Hereby, the same potential can be selected at several iteration steps, which is not a problem.)
By construction, the interatomic potentials of the subset use optimal polynomial degrees or, in other words, are adjusted to describe optimally and efficiently the fitted data. The subset contains a dramatically reduced number of potentials with respect to the initial set of all physically reasonable degree combinations. We further use this subset to manually find the final interatomic potential $\Phi(T_{\mathrm{e}})$ which exhibits at all studied electronic temperatures $T_{\mathrm{e}}$'s the properties: Reproducing the phonon bandstructure of the diamond structure, reproducing the cohesive energy curves of the diamond, sc, fcc and bcc structures and reproducing the atomic root-mean-square displacements of bulk Si after an increase of $T_{\mathrm{e}}$ for at least 1 ps.

# 3 Electronic temperature-dependent potential coefficients

Our potential uses the polynomial degrees

$$N_2^{(r)} = 10, \qquad N_3^{(r)} = 3, \qquad N_3^{(\theta)} = 3 \qquad N_\rho^{(\rho)} = 2, \qquad N_\rho^{(r)} = 2 \tag{3}$$

and needs therefore in total 23 coefficients. The two-body term $\Phi_2$ has 9, the three-body term $\Phi_3$ has 12, and the embedding function $\Phi_\rho$ has 2 coefficients. Furthermore, the cutoff radii

$$r_2^{(\mathrm{c})} = 0.63 \text{ nm}, \qquad r_3^{(\mathrm{c})} = 0.42 \text{ nm}, \qquad r_\rho^{(\mathrm{c})} = 0.48 \text{ nm} \tag{4}$$

are constant and do not depend on the electronic temperature $T_{\mathrm{e}}$. The $T_{\mathrm{e}}$-dependence of the coefficients was fitted to a polynomial of degree 5. Hence, any coefficient $c$ of the potential depends on $T_{\mathrm{e}}$ as

$$c = \sum_{k=0}^{5} a^{(k)} \left( \frac{T_{\mathrm{e}}}{31577\,\mathrm{K}} \right)^k . \tag{5}$$

In order to describe the parametrization of the term $\Phi_0$, let us consider an isolated atom. It contains discrete energy levels of the electrons. The electronic occupation of these energy levels is given by a Fermi distribution with $T_{\mathrm{e}}$. Since there exists a gap between the highest occupied and the first unoccupied level, the internal energy $U_0$ and the entropy $S_0$ of the atom does not change with increasing $T_{\mathrm{e}}$ at low $T_{\mathrm{e}}$'s. Consequently, the Helmholtz free energy

$$\Phi_0(T_{\mathrm{e}}) = U_0 - T_{\mathrm{e}}\, S_0 \tag{6}$$

of the isolated atom is a linear function of $T_{\mathrm{e}}$ at low $T_{\mathrm{e}}$'s. Starting from $\sim$ 4500 K, a significant occupation occurs in the first unoccupied level and the internal energy $U_0$ and the entropy $S_0$ start depending on $T_{\mathrm{e}}$. Above this temperature, the Helmholtz free energy $\Phi_0(T_{\mathrm{e}})$ behaves in a non-linear fashion. Hence, the Helmholtz free energy $\Phi_0$ of an isolated atom is fitted to a polynomial of degree 1 at $T_{\mathrm{e}} \leq 4500$ K and to a polynomial of degree

13 at $T_e > 4500$ K:

$$\Phi_0 = \begin{cases} a_0^{(0)} + a_0^{(1)} \left(\frac{T_e - 4500\,\mathrm{K}}{31577\,\mathrm{K}}\right) & T_e \leq 4500\,\mathrm{K} \\ a_0^{(0)} + a_0^{(1)} \left(\frac{T_e - 4500\,\mathrm{K}}{31577\,\mathrm{K}}\right) + \sum_{k=4}^{13} a_0^{(k)} \left(\frac{T_e - 4500\,\mathrm{K}}{31577\,\mathrm{K}}\right)^k & T_e > 4500\,\mathrm{K}. \end{cases} \quad (7)$$

The corresponding plots are presented in Sec. 4.4. By construction, $\Phi_0$, its first, second, and third derivative are continuous functions of $T_e$.
The parametrization of the potential is tabulated in Tab. 1 - 4. The unit of the coefficients is eV and the unit of $T_e$ is K. The fitted range of the polynomial expansion yields 316 K $\leq T_e \leq$ 31577 K.

**Table 1:** Parametrization of $c_2^{(q)} = \sum_{k=0}^{5} a_2^{(k\,q)} \left(\frac{T_e}{31577\,\mathrm{K}}\right)^k$ for the two-body term $\Phi_2$, see eq. (2) in the main paper.

| $k$ | $q$ | $a_2^{(k\,q)}$ | $k$ | $q$ | $a_2^{(k\,q)}$ | $k$ | $q$ | $a_2^{(k\,q)}$ |
|---|---|---|---|---|---|---|---|---|
| 0 | 2 | -0.652029301662623 | 0 | 3 | -19.0589296869611 | 0 | 4 | 546.769257376815 |
| 1 | 2 | 9.26314534875668 | 1 | 3 | -400.089680112155 | 1 | 4 | 6319.96355713893 |
| 2 | 2 | -50.0186051618631 | 2 | 3 | 2167.05447438595 | 2 | 4 | -35385.6550126843 |
| 3 | 2 | 115.557349548295 | 3 | 3 | -4520.34437699249 | 3 | 4 | 71794.8635849514 |
| 4 | 2 | -114.529669723874 | 4 | 3 | 4095.42902709553 | 4 | 4 | -62858.4678911266 |
| 5 | 2 | 40.7054174379305 | 5 | 3 | -1352.35365149216 | 5 | 4 | 20099.4017864489 |
| 0 | 5 | -5494.99348657106 | 0 | 6 | 27386.1918081797 | 0 | 7 | -75861.4334859187 |
| 1 | 5 | -48814.0360404613 | 1 | 6 | 210387.578621541 | 1 | 7 | -529386.428965916 |
| 2 | 5 | 283940.662885404 | 2 | 6 | -1261022.76787976 | 2 | 7 | 3245873.44871437 |
| 3 | 5 | -573728.968470894 | 3 | 6 | 2555763.80515297 | 3 | 7 | -6616167.17139263 |
| 4 | 5 | 496377.262929330 | 4 | 6 | -2204123.17465255 | 4 | 7 | 5709449.19416504 |
| 5 | 5 | -156654.734823045 | 5 | 6 | 692217.214417601 | 5 | 7 | -1791097.75814672 |
| 0 | 8 | 119482.732077564 | 0 | 9 | -101003.484900608 | 0 | 10 | 35858.0271585324 |
| 1 | 8 | 775653.843416637 | 1 | 9 | -614687.832893782 | 1 | 10 | 203955.905899671 |
| 2 | 8 | -4831404.94060070 | 2 | 9 | 3865581.63043600 | 2 | 10 | -1288401.57956179 |
| 3 | 8 | 9911649.99101982 | 3 | 9 | -7978309.71558179 | 3 | 10 | 2672708.20259957 |
| 4 | 8 | -8574228.73882666 | 4 | 9 | 6923565.00773351 | 4 | 10 | -2326924.03159739 |
| 5 | 8 | 2692171.33820813 | 5 | 9 | -2178041.48087368 | 5 | 10 | 733755.194711132 |

**Table 2:** Parametrization of $c_3^{(q_1\,q_2\,q_3)} = \sum_{k=0}^{5} a_3^{(k\,q_1\,q_2\,q_3)} \left(\frac{T_e}{31577\,\mathrm{K}}\right)^k$ for the three-body term $\Phi_3$, see eq. (3) in the main paper.

| $k$ | $q_1$ | $q_2$ | $q_3$ | $a_3^{(k\,q_1\,q_2\,q_3)}$ | $k$ | $q_1$ | $q_2$ | $q_3$ | $a_3^{(k\,q_1\,q_2\,q_3)}$ |
|---|---|---|---|---|---|---|---|---|---|
| 0 | 2 | 2 | 0 | -0.484742122936188 | 0 | 2 | 3 | 0 | 10.9087150193338 |
| 1 | 2 | 2 | 0 | -9.06449732747187 | 1 | 2 | 3 | 0 | 32.6476593724955 |
| 2 | 2 | 2 | 0 | 41.9525344564407 | 2 | 2 | 3 | 0 | -234.821794328009 |
| 3 | 2 | 2 | 0 | -73.0549723173192 | 3 | 2 | 3 | 0 | 445.128565939339 |
| 4 | 2 | 2 | 0 | 62.1731314312558 | 4 | 2 | 3 | 0 | -384.590065348177 |
| 5 | 2 | 2 | 0 | -20.9735149728352 | 5 | 2 | 3 | 0 | 128.088250726806 |
| 0 | 3 | 3 | 0 | -29.0228451088965 | 0 | 2 | 2 | 1 | 22.1886312645380 |
| 1 | 3 | 3 | 0 | -20.4131309827352 | 1 | 2 | 2 | 1 | -35.1166767655775 |
| 2 | 3 | 3 | 0 | 338.473408313579 | 2 | 2 | 2 | 1 | -105.001706438450 |
| 3 | 3 | 3 | 0 | -686.718447255702 | 3 | 2 | 2 | 1 | 325.429922575188 |
| 4 | 3 | 3 | 0 | 593.638243677844 | 4 | 2 | 2 | 1 | -302.151293271689 |
| 5 | 3 | 3 | 0 | -193.368789264996 | 5 | 2 | 2 | 1 | 96.1147759289952 |
| 0 | 2 | 3 | 1 | -120.252372821342 | 0 | 3 | 3 | 1 | 168.069490773212 |
| 1 | 2 | 3 | 1 | 159.047356694074 | 1 | 3 | 3 | 1 | -161.910998601428 |
| 2 | 2 | 3 | 1 | 749.046048760271 | 2 | 3 | 3 | 1 | -1315.34984931164 |
| 3 | 2 | 3 | 1 | -2216.09205938898 | 3 | 3 | 3 | 1 | 3702.73203746780 |
| 4 | 2 | 3 | 1 | 2126.62367753068 | 4 | 3 | 3 | 1 | -3605.91631090411 |
| 5 | 2 | 3 | 1 | -707.455756431839 | 5 | 3 | 3 | 1 | 1228.41451611926 |
| 0 | 2 | 2 | 2 | -19.4315027093624 | 0 | 2 | 3 | 2 | 96.3144087590581 |
| 1 | 2 | 2 | 2 | 42.1788604704338 | 1 | 2 | 3 | 2 | -173.588114464854 |
| 2 | 2 | 2 | 2 | 9.67634296126227 | 2 | 2 | 3 | 2 | -157.818542202707 |
| 3 | 2 | 2 | 2 | -141.700074704502 | 3 | 2 | 3 | 2 | 751.291373937404 |
| 4 | 2 | 2 | 2 | 157.523635751903 | 4 | 2 | 3 | 2 | -702.941624093910 |
| 5 | 2 | 2 | 2 | -54.5952459846017 | 5 | 2 | 3 | 2 | 212.581414043121 |
| 0 | 3 | 3 | 2 | -77.3561827130667 | 0 | 2 | 2 | 3 | -65.4726886857960 |
| 1 | 3 | 3 | 2 | 156.577143486935 | 1 | 2 | 2 | 3 | 102.053920198204 |
| 2 | 3 | 3 | 2 | 314.860740984096 | 2 | 2 | 2 | 3 | 425.612227408026 |
| 3 | 3 | 3 | 2 | -1179.99411420945 | 3 | 2 | 2 | 3 | -1403.05615543312 |
| 4 | 3 | 3 | 2 | 1097.63560691297 | 4 | 2 | 2 | 3 | 1437.50728878185 |
| 5 | 3 | 3 | 2 | -335.520618998547 | 5 | 2 | 2 | 3 | -504.993626721485 |
| 0 | 2 | 3 | 3 | 336.447897505456 | 0 | 3 | 3 | 3 | -420.786323757512 |
| 1 | 2 | 3 | 3 | -507.178567927645 | 1 | 3 | 3 | 3 | 602.981897592014 |
| 2 | 2 | 3 | 3 | -2093.07884553079 | 2 | 3 | 3 | 3 | 2804.76991700882 |
| 3 | 2 | 3 | 3 | 6834.03239451122 | 3 | 3 | 3 | 3 | -8941.73384478093 |
| 4 | 2 | 3 | 3 | -6988.05320202182 | 4 | 3 | 3 | 3 | 9095.82514910275 |
| 5 | 2 | 3 | 3 | 2453.90944239108 | 5 | 3 | 3 | 3 | -3187.19934480896 |

**Table 3:** Parametrization of $c_\rho^{(q_1\,q_2)} = \sum_{k=0}^{5} a_\rho^{(k\,q_1\,q_2)} \left(\frac{T_e}{31577\,\mathrm{K}}\right)^k$ for the embedding function $\Phi_\rho$, see eq. (5) in the main paper.

| $k$ | $q_1$ | $q_2$ | $a_\rho^{(k\,q_1\,q_2)}$ | $k$ | $q_1$ | $q_2$ | $a_\rho^{(k\,q_1\,q_2)}$ |
|---|---|---|---|---|---|---|---|
| 0 | 1 | 2 | -14.1226298367901 | 0 | 2 | 2 | 15.1973595898918 |
| 1 | 1 | 2 | 42.8178754251152 | 1 | 2 | 2 | -76.2426696199033 |
| 2 | 1 | 2 | -46.9725273143709 | 2 | 2 | 2 | 180.466580679766 |
| 3 | 1 | 2 | -7.49328100982082 | 3 | 2 | 2 | -227.822610054901 |
| 4 | 1 | 2 | 50.9341743266501 | 4 | 2 | 2 | 143.162975148651 |
| 5 | 1 | 2 | -26.0690457870547 | 5 | 2 | 2 | -34.7706099024473 |

**Table 4:** Parametrization of the Helmholtz free energy of an isolated atom $\Phi_0$, see eq. (7).

| $k$ | $a_0^{(k)}$ | $k$ | $a_0^{(k)}$ | $k$ | $a_0^{(k)}$ |
|---|---|---|---|---|---|
| 0 | -102.905307363449 | 1 | -10.3921123486934 | 4 | -1.06389593948069 |
| 5 | 12.4244554652269 | 6 | -183.607940058980 | 7 | 816.889082583121 |
| 8 | -1946.46133504029 | 9 | 2899.84763931852 | 10 | -2817.24323376719 |
| 11 | 1750.31164692968 | 12 | -635.201199559016 | 13 | 102.801048351004 |

# 4 Physical properties calculated using the developed interatomic potential

# Comparison with *ab initio* calculations using CHIVES

## 4.1 Atomic root mean-square displacements in $z$-direction

To verify the description of the laser-induced expansion of the Si thin-film, we perform the MD simulations of the thin-film at various electronic temperatures $T_e$'s. Both *ab initio* and classical MD simuations start with the same initial conditions. To get a measure of the expansion, we calculated the evolution of atomic root mean-square displacements in $z$-direction, $\mathrm{RMSD}_z(t)$, from our *ab initio* and classical simulations and present the corresponding curves in Fig. 1. $\mathrm{RMSD}_z(t)$ is accurately described by the potential, which indicates that the laser-induced expansion of the thin-film is reasonably modeled by the potential.

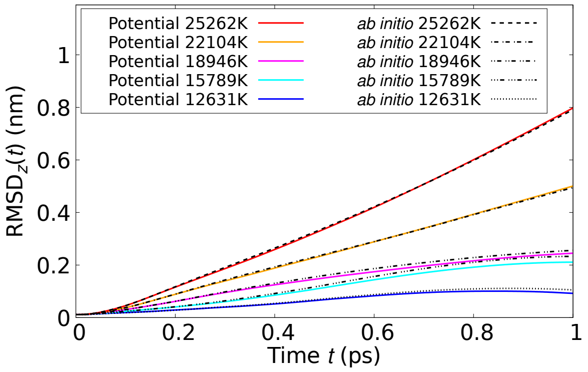


**Figure 1:** Time-dependent atomic root mean-square displacements in $z$-direction $\mathrm{RMSD}_z(t)$ of the thin-film are shown at various $T_\mathrm{e}$'s. The black dashed lines correspond to *ab initio* and the colored lines to the potential.

## 4.2 Relative error in forces determined in independent MD simulation runs

Four additional independent samples at room temperature $T_\mathrm{i} = 300$ K were prepared for the thin-film using the Andersen thermostat. Using these initializations, classical MD simulations of laser excitation were repeated at various $T_\mathrm{e}$'s. For these additional runs and the fitted run, the relative force error of the potential (*cf.* second term for $s = 1$ in eq. (6) in the main paper)

$$f_\mathrm{err} = \sqrt{\frac{\sum_t \sum_i \left| -\nabla_{\mathbf{r}_i} \Phi\left(\left\{\mathbf{r}_j(t)\right\}\right) - \mathbf{f}_i(t) \right|^2}{\sum_t \sum_i \left|\mathbf{f}_i(t)\right|^2}} \tag{8}$$

was determined. Hereby $\mathbf{f}_i(t)$ denotes the *ab initio* force acting on atom $i$ and $\left\{\mathbf{r}_j(t)\right\}$ the atomic coordinates. The obtained relative force errors of the different runs at various $T_\mathrm{e}$'s are shown in Tab. 5.

**Table 5:** Relative force error in the thin-film MD simulation at constant $T_\mathrm{e}$ is listed for the different independent runs. Only run 1 was used for fitting.

| $T_\mathrm{e}$ (mHa) | $T_\mathrm{e}$ (K) | run 1 $f_\mathrm{err}$ (%) | run 2 $f_\mathrm{err}$ (%) | run 3 $f_\mathrm{err}$ (%) | run 4 $f_\mathrm{err}$ (%) | run 5 $f_\mathrm{err}$ (%) |
|---|---|---|---|---|---|---|
| 40 | 12631 | 7.7 | 7.6 | 7.4 | 7.5 | 7.8 |
| 50 | 15789 | 7.3 | 7.1 | 7.1 | 7.2 | 7.5 |
| 60 | 18946 | 11.2 | 11.1 | 11.0 | 10.7 | 11.8 |
| 70 | 22104 | 8.9 | 9.0 | 9.2 | 8.8 | 8.9 |
| 80 | 25262 | 6.6 | 6.7 | 6.7 | 6.7 | 6.7 |

Run 1 was used for the potential development. One can see that the potential describes

the atomic forces in the independent runs at the same level of accuracy. This indicates that fitting additional independent *ab initio* runs should not produce any improvement of the potential.

### 4.3 Absorbed energy of the electrons in the bulk

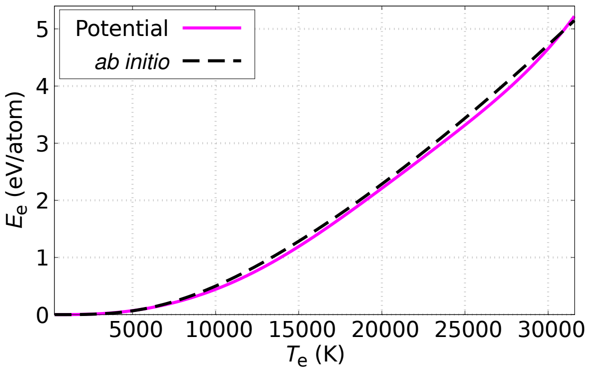


**Figure 2:** Energy absorbed by the electrons $E_\mathrm{e}$ as a function of $T_\mathrm{e}$ for the ideal diamond structure.

The presented classical interatomic potential $\Phi(T_\mathrm{e})$ corresponds to the Helmholtz free energy. Hence, one can derive the internal energy of the electrons $U_\mathrm{e}$ using thermodynamic relations

$$U_\mathrm{e}(T_\mathrm{e}) = \Phi(T_\mathrm{e}) - T_\mathrm{e}\,\frac{\partial\Phi(T_\mathrm{e})}{\partial T_\mathrm{e}}. \qquad (9)$$

Therefore, the energy absorbed by the electrons can be calculated from this equation as

$$E_\mathrm{e}(T_\mathrm{e}) = U_\mathrm{e}(T_\mathrm{e}) - U_\mathrm{e}(316\ \mathrm{K}). \qquad (10)$$

Fig. 2 shows $E_\mathrm{e}(T_\mathrm{e})$ for the ideal diamond structure derived from our potential and from *ab initio* and indicates that $E_\mathrm{e}$ is accurately described by the potential.

### 4.4 Electronic absorbed energy and specific heat of an isolated atom

We also calculated the absorbed energy and the specific heat of the electrons as a function of $T_\mathrm{e}$ for a single atom (see Fig. 3 and Fig. 4, respectively).

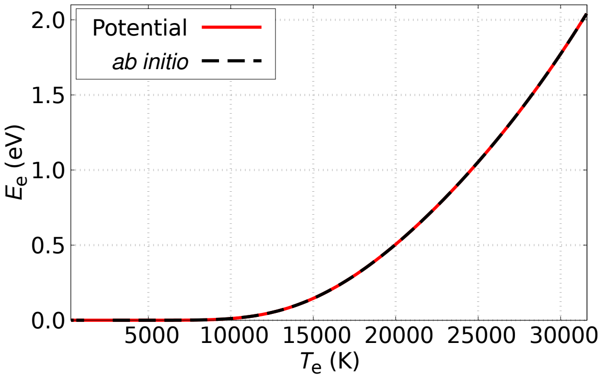


**Figure 3:** Energy absorbed by the electrons $E_\mathrm{e}$ as a function of $T_\mathrm{e}$ for an isolated atom.

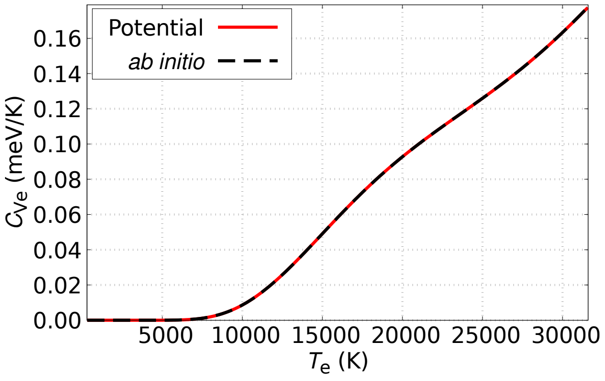


**Figure 4:** Specific heat of the electrons $C_{\mathrm{Ve}}$ as a function of $T_\mathrm{e}$ for an isolated atom.

## 4.5 Elastic constants

We verified the description of the independent elastic constants $C_{11}, C_{12}, C_{44}$ in bulk laser-excited and not excited Si. For this, we calculated the elastic constants from the derivatives of the acoustic phonon branches at the Γ-Point [3]. We present the relative differences

$$\Delta C_{11} = \frac{\left|C_{11}^{(\Phi)} - C_{11}^{(ab\ initio)}\right|}{\left|C_{11}^{(ab\ initio)}\right|}, \quad \Delta C_{12} = \frac{\left|C_{12}^{(\Phi)} - C_{12}^{(ab\ initio)}\right|}{\left|C_{12}^{(ab\ initio)}\right|}, \quad \Delta C_{44} = \frac{\left|C_{44}^{(\Phi)} - C_{44}^{(ab\ initio)}\right|}{\left|C_{44}^{(ab\ initio)}\right|} \tag{11}$$

between the elastic constants derived from the potential and those derived from the *ab initio* calculations in Tab. 6.

**Table 6:** Relative errors $\Delta C_{11}, \Delta C_{12}, \Delta C_{44}$ in the independent elastic constants $C_{11}, C_{12}, C_{44}$ derived from the potential and from *ab initio* at various electronic temperatures $T_e$'s.

| $T_e$ (mHa) | $T_e$ (K) | $\Delta C_{11}$ (%) | $\Delta C_{12}$ (%) | $\Delta C_{44}$ (%) |
|---|---|---|---|---|
| 1 | 316 | -7.6 | -56.1 | -17.5 |
| 10 | 3158 | -1.3 | -73.0 | -18.9 |
| 20 | 6315 | 2.7 | -104.1 | -15.3 |
| 30 | 9473 | 6.8 | -575.4 | -10.4 |
| 40 | 12631 | 8.6 | 67.2 | -6.6 |
| 50 | 15789 | 7.7 | 18.5 | -4.0 |
| 60 | 18946 | 5.2 | 5.7 | -3.3 |
| 70 | 22104 | 2.0 | -3.6 | 35.4 |
| 80 | 25262 | -1.2 | -28.1 | 23.1 |
| 90 | 28420 | -4.4 | -149.4 | 28.1 |
| 100 | 31577 | -7.6 | 609.2 | 27.4 |

For electronic temperatures $T_e$'s above 60 mHa, the derivatives of the acoustic phonon branches become negative for both, *ab initio* and potential. Hence, the elastic constants may not be properly defined any more above this electronic temperature. In general, the values of the elastic constants show a reasonable agreement.

## 4.6 Pair-correlation function and bond angle distribution

We verified the description of the pair-correlation function and the bond angle distribution between the neighboring atoms in bulk Si during the laser excitation. For this, we took the initial conditions of our previously published *ab initio* MD simulations of laser-induced nonthermal melting at 58 mHa (18315 K), 60 mHa (18946 K), 70 mHa (22104 K) and 80 mHa (25262 K) from [4] and of laser-induced thermal phonon squeezing at 50 mHa (15789 K) from [5], and repeated the simulations with the new classical potential. Figs. 5, 7, 9 show typical pair-correlation functions obtained from the simulations 1 ps after the laser irradiation. In the same way, Figs. 6, 8, 10 present typical bond angle distributions. For

the latter, atoms were taken into account up to a distance of 0.41 nm. Our results show, that at least for the simulated time of 1 ps, the pair-correlation function and bond angle distribution are reliably described by the potential.

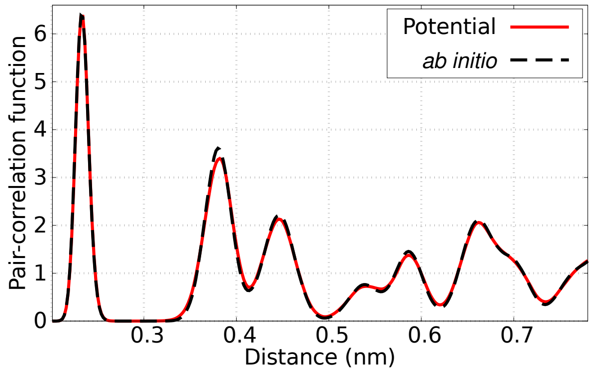


**Figure 5:** Pair-correlation function 1 ps after the laser excitation at $T_\mathrm{e}$=50 mHa.

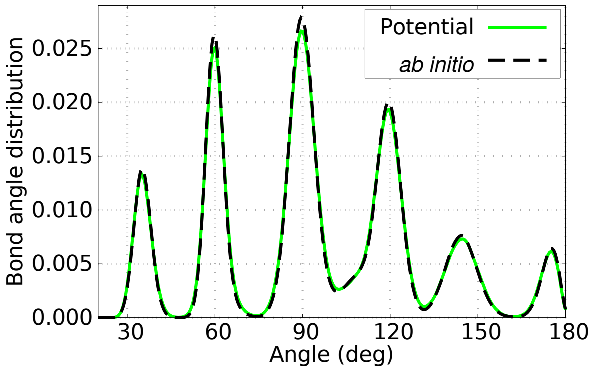


**Figure 6:** Bond angle distribution 1 ps after the laser excitation at $T_\mathrm{e}$=50 mHa.

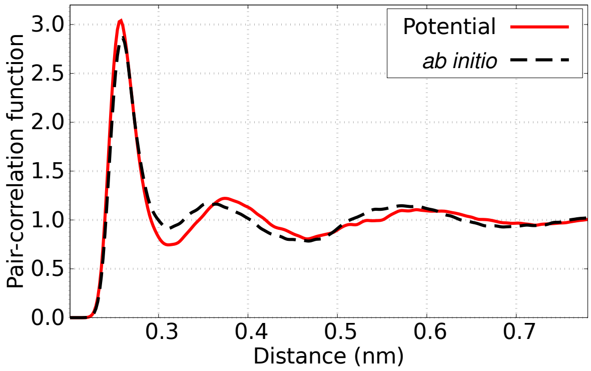


**Figure 7:** Pair-correlation function 1 ps after the laser excitation at $T_\mathrm{e}$=58 mHa.

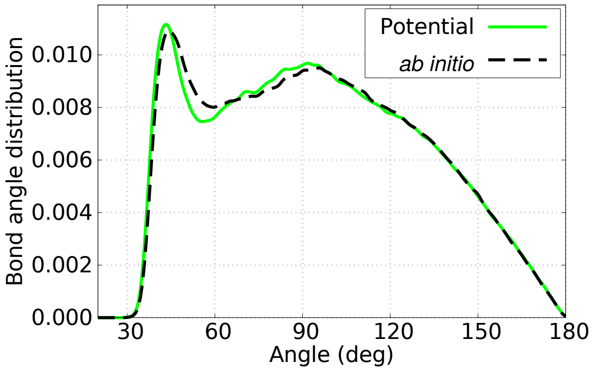


**Figure 8:** Bond angle distribution 1 ps after the laser excitation at $T_\mathrm{e}$=58 mHa.

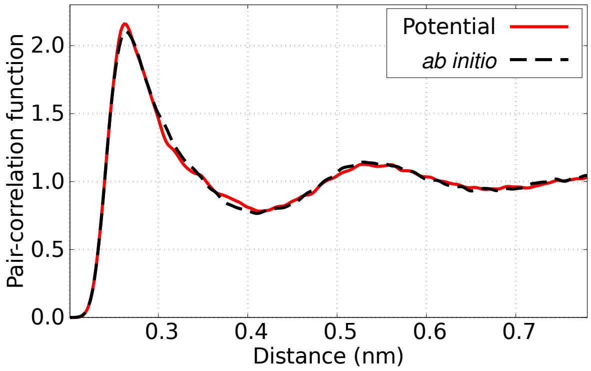


**Figure 9:** Pair-correlation function 1 ps after the laser excitation at $T_\mathrm{e}$=70 mHa.

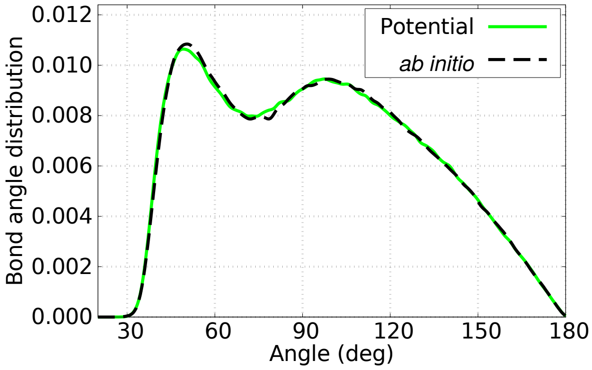


**Figure 10:** Bond angle distribution 1 ps after the laser excitation at $T_\mathrm{e}$=70 mHa.

# 5 Fortran implementation of the developed interatomic potential

The file `calc_Si_Phi_of_Te_module.f90` contains a Fortran subroutine, which calculates the forces and the Helmholtz free structural energy of an ensemble of atoms from our potential at a given electronic temperature $T_\mathrm{e}$. The subroutine reads the input variables `NumAt, MaxNumNeib, PBC, BoxLength, coord, Te` and sets the output variables `force, energy, info` without using any global variables. In the following, we list the meaning of selected internal program variables:

`Nr2` $\triangleq N_2^{(r)}$, `Nr3` $\triangleq N_3^{(r)}$, `Nt3` $\triangleq N_3^{(\theta)}$, `Nrhorho` $\triangleq N_\rho^{(\rho)}$, `Nrrho` $\triangleq N_\rho^{(r)}$,

`Rc2` $\triangleq r_2^{(\mathrm{c})}$, `Rc3` $\triangleq r_3^{(\mathrm{c})}$, `Rcrho` $\triangleq r_\rho^{(\mathrm{c})}$, `mIRc2` $\triangleq -1/r_2^{(\mathrm{c})}$, `mIRc3` $\triangleq -1/r_3^{(\mathrm{c})}$,

`mIRcrho` $\triangleq -1/r_\rho^{(\mathrm{c})}$, `maxRc` $\triangleq \max\left(r_2^{(\mathrm{c})}, r_3^{(\mathrm{c})}, r_\rho^{(\mathrm{c})}\right)$, `maxRc2` $\triangleq \max\left(r_2^{(\mathrm{c})}, r_3^{(\mathrm{c})}, r_\rho^{(\mathrm{c})}\right)^2$,

`rhoi(q2)` $\triangleq \rho_i^{(q_2)}$, `arhoipower(q1,q2)` $\triangleq \left(\frac{\rho_i^{(q_2)}}{1+\rho_i^{(q_2)}}\right)^{q_1}$, `cosijk` $\triangleq \cos(\theta_{ijk})$,

`cosijkpower(q3)` $\triangleq \cos(\theta_{ijk})^{q_3}$, `rij` $\triangleq r_{ij}$, `rik` $\triangleq r_{ik}$, `Irij` $\triangleq 1/r_{ij}$, `Irik` $\triangleq 1/r_{ik}$.

# References


[1] H. C. Andersen, *Molecular dynamics simulations at constant pressure and/or temperature*, The Journal of Chemical Physics **72**, 2384–2393, 1980.

[2] E. Bitzek, P. Koskinen, F. Gähler, M. Moseler and P. Gumbsch, *Structural Relaxation Made Simple*, PRL **67**, 170201, 2006.

[3] R. Gross, A. Marx, *Festkörperphysik*, Oldenbourg Verlag München, (2012).

[4] E. S. Zijlstra, A. Kalitsov, T. Zier, and M. E. Garcia, *Fractional Diffusion in Silicon*, Advanced Materials **25**, 5605 (2013).

[5] E. S. Zijlstra, A. Kalitsov, T. Zier, and M. E. Garcia, *Squeezed Thermal Phonons Precurse Nonthermal Melting of Silicon as a Function of Fluence*, Phys. Rev. X **3**, 011005 (2013).
